# Supplementary material for: Can Graph Learning Improve Planning in LLM-based Agents?
Source: arXiv:2405.19119 source file (2024-10-26)
Supplement: Supplementary file 1 [file impacts.tex]

\section{Broader Impacts}\label{sec:impacts}
In this paper, we did not use any non-public data, unauthorized
software, or API in our paper, there are no privacy or other related ethical concerns. Similar to other models designed for autonomous agents, our model also has the unfortunate potential to be used for malicious attacks. We pledge to restrict the usage of our model exclusively to the realm of research to prevent such misuse.
